# Supplementary material for: ChatGPT Beyond English: Towards a Comprehensive Evaluation of Large Language Models in Multilingual Learning
Source: arXiv:2304.05613 source file (2023-04-12)
Supplement: Supplementary file 1 [file section-appendix.tex]

\clearpage
\onecolumn

\section{Language-specific Prompts}

\newcommand{\mtr}[2]{\multirow{#1}{*}{#2}}

This section provides language-specific prompts that have been used in our experiments. Note that these prompts are obtained by translating the original human-designed English versions into specific languages. Tables \ref{tab:prompt-xglue-pos}, \ref{tab:prompt-multiconer}, and \ref{tab:prompt-smiler} show language-specific prompts for the POS Tagging, Named Entity Recognition, and Relation Classification tasks. We use ChatGPT to translate English prompts to target language prompts with label-preservation constraints so that the output prompts can retain the original label notations from each dataset (all translated prompts are back-translated using Google Translate for validation).

Our language-specific prompts for other tasks, i.e., Natural Language Inference, Question Answering, Common Sense Reasoning, and Summarization, are directly translated from English versions using Google Translate, as demonstrated in Tables \ref{tab:prompt-xnli}, \ref{tab:prompt-xquad}, \ref{tab:prompt-xcsqa}, \ref{tab:propmpt-indic}, and \ref{tab:prompt-xlsum}.

\begin{table}[!h]
\centering
\resizebox{\textwidth}{!}{
\begin{tabular}{p{1.5cm} p{25.5cm}}
\hline
    \mtctt{1}{Language} & \mtctt{1}{Task Description} \\
    \hline
    \mtr{4}{English} & Please provide the POS tags for each word in the input sentence. The input sentence will be a list of each word in the sentence. The output format should be a list of tuples, where each tuple consists of a word from the input text and its corresponding POS tag label from the tag label set: ['ADJ', 'ADP', 'ADV', 'AUX', 'CCONJ', 'DET', 'INTJ', 'NOUN', 'NUM', 'PART', 'PRON', 'PROPN', 'PUNCT', 'SCONJ', 'SYM', 'VERB', 'X']. \\ \hline
    \mtr{4}{German} & Bitte geben Sie die POS-Tags für jedes Wort im Eingabesatz an. Der Eingabesatz ist eine Liste aller Wörter eines Satzes. Das Ausgabeformat sollte eine Liste von Tupeln sein, wobei jedes Tupel aus einem Wort aus dem Eingabetext und seinem entsprechenden POS-Tag-Label aus dem Tag-Label-Set besteht: ['ADJ', 'ADP', 'ADV', 'AUX', 'CCONJ', 'DET', 'INTJ', 'NOUN', 'NUM', 'PART', 'PRON', 'PROPN', 'PUNCT', 'SCONJ', 'SYM', 'VERB', 'X ']. \\ \hline
    \mtr{4}{Spanish} & Proporcione las etiquetas POS para cada palabra en la oración de entrada. La oración de entrada será una lista de cada palabra en una oración. El formato de salida debe ser una lista de tuplas, donde cada tupla consta de una palabra del texto de entrada y su etiqueta de etiqueta POS correspondiente del conjunto de etiquetas de etiquetas: ['ADJ', 'ADP', 'ADV', 'AUX', 'CCONJ', 'DET', 'INTJ', 'NOUN', 'NUM', 'PARTE', 'PRON', 'PROPN', 'PUNCT', 'SCONJ', 'SYM', 'VERB', 'X ']. \\ \hline
    \mtr{4}{Dutch} & Geef de POS-tags op voor elk woord in de invoerzin. De invoerzin is een lijst van elk woord in een zin. Het uitvoerformaat moet een lijst met tupels zijn, waarbij elke tupel bestaat uit een woord uit de invoertekst en het bijbehorende POS-taglabel uit de taglabelset: ['ADJ', 'ADP', 'ADV', 'AUX', 'CCONJ', 'DET', 'INTJ', 'NOUN', 'NUM', 'PART', 'PRON', 'PROPN', 'PUNCT', 'SCONJ', 'SYM', 'VERB', 'X ']. \\ \hline
    \mtr{5}{Bulgarian} & \foreignlanguage{bulgarian}{Моля, предоставете POS етикетите за всяка дума във въведеното изречение. Въведеното изречение ще бъде списък на всяка дума в изречение. Изходният формат трябва да бъде списък от кортежи, където всеки кортеж се състои от дума от входния текст и съответния етикет на POS етикет от набора етикети на етикети: ['ADJ', 'ADP', 'ADV', 'AUX', 'CCONJ', 'DET', 'INTJ', 'NOUN', 'NUM', 'PART', 'PRON', 'PROPN', 'PUNCT', 'SCONJ', 'SYM', 'VERB', 'X ']. }\\ \hline
    \mtr{4}{French} & Veuillez fournir les balises POS pour chaque mot dans la phrase d'entrée. La phrase d'entrée sera une liste de chaque mot d'une phrase. Le format de sortie doit être une liste de tuples, où chaque tuple consiste en un mot du texte d'entrée et son étiquette de balise POS correspondante de l'ensemble d'étiquettes de balise : ['ADJ', 'ADP', 'ADV', 'AUX', 'CCONJ', 'DET', 'INTJ', 'NOUN', 'NUM', 'PART', 'PRON', 'PROPN', 'PUNCT', 'SCONJ', 'SYM', 'VERB', 'X ']. \\ \hline
    \mtr{4}{Polish} & Podaj tagi POS dla każdego słowa we wprowadzanym zdaniu. Zdanie wejściowe będzie listą każdego słowa w zdaniu. Format wyjściowy powinien być listą krotek, gdzie każda krotka składa się ze słowa z tekstu wejściowego i odpowiadającej mu etykiety znacznika POS z zestawu etykiet znaczników: ['ADJ', 'ADP', 'ADV', 'AUX', „CCONJ”, „DET”, „INTJ”, „RZECZOW.”, „LICZBA”, „CZĘŚĆ”, „PRON”, „PROPN”, „PUNCT”, „SCONJ”, „SYM”, „CZASOWNIK”, „X ']. \\ \hline
    \mtr{3}{Turkish} & Lütfen giriş cümlesindeki her kelime için POS etiketlerini sağlayın. Giriş cümlesi, bir cümledeki her kelimenin bir listesi olacaktır. Çıktı formatı, her bir demetin giriş metnindeki bir kelimeden ve etiket etiket kümesinden karşılık gelen POS etiketinden oluştuğu bir demetler listesi olmalıdır: ['ADJ', 'ADP', 'ADV', 'AUX', 'CCONJ', 'DET', 'INTJ', 'İSİM', 'NUM', 'BÖLÜM', 'ZAMİR', 'PROPN', 'PUNCT', 'SCONJ', 'SYM', 'VERB', 'X ']. \\ \hline
    \mtr{4}{Italian} & ornisci i tag POS per ogni parola nella frase di input. La frase di input sarà un elenco di ogni parola su una frase. Il formato di output dovrebbe essere un elenco di tuple, in cui ogni tupla è composta da una parola del testo di input e dalla corrispondente etichetta del tag POS dal set di etichette del tag: ['ADJ', 'ADP', 'ADV', 'AUX', 'CCONJ', 'DET', 'INTJ', 'NOUN', 'NUM', 'PART', 'PRON', 'PROPN', 'PUNCT', 'SCONJ', 'SYM', 'VERB', 'X ']. \\ \hline
    \mtr{4}{Arabic} & \foreignlanguage{arabic}{ يرجى تقديم علامات POS لكل كلمة في جملة الإدخال. ستكون جملة الإدخال قائمة بكل كلمة في الجملة. يجب أن يكون تنسيق الإخراج عبارة عن قائمة من المجموعات ، حيث تتكون كل مجموعة من كلمة من نص الإدخال وتسمية علامة POS المقابلة لها من مجموعة تصنيف العلامات:} \\
    & ['ADJ'، 'ADP'، 'ADV'، 'AUX'، 'CCONJ'، 'DET'، 'INTJ'، 'NOUN'، 'NUM'، 'PART'، 'PRON'، 'PROPN'، 'PUNCT'، 'SCONJ'، 'SYM'، 'VERB'، 'X'] \\
    & \foreignlanguage{arabic}{ ربما توجد جمل إدخال متعددة ، يجب أن تكون المخرجات قائمة متعددة من المجموعات وفقًا لذلك.  يجب أن تتضمن إجابتك قائمة المجموعات فقط ، بالترتيب الذي تظهر به الكلمات في جملة الإدخال ، مع احتواء كل مجموعة على تسمية علامة نقطة البيع المقابلة لـ تلك الكلمة. } \\ \hline
\end{tabular}
}
\caption{Language-specific task descriptions for the XGLUE-POS dataset translated from the English version.}
\label{tab:prompt-xglue-pos}
\end{table}

\begin{table}[!h]
\centering
\resizebox{\textwidth}{!}{
\begin{tabular}{p{1.5cm} p{24cm}}
    \hline
    & \\
    \mtctt{1}{Language} & \mtctt{1}{Task Description} \\
    &  \\
    \hline
    \mtr{5}{English} & You are working as a named entity recognition expert and your task is to label a given text with named entity labels. Your task is to identify and label any named entities present in the text. The named entity labels that you will be using are PER (person), LOC (location), CORP (corporation), CW (creative work), GRP (group of people), and PROD (product). You may encounter multi-word entities, so make sure to label each word of the entity with the appropriate prefix ('B' for the first word of the entity, 'I' for any non-initial word of the entity). For words which are not part of any named entity, you should return 'O'. Your output format should be a list of tuples, where each tuple consists of a word from the input text and its corresponding named entity label. \\ \hline
    \mtr{5}{German} & ie arbeiten als Expertin für benannte Entitäten (Named Entity Recognition) und Ihre Aufgabe besteht darin, einen gegebenen Text mit benannten Entitäten zu kennzeichnen. Ihre Aufgabe ist es, alle benannten Entitäten im Text zu identifizieren und zu kennzeichnen. Die benannten Entitätslabels, die Sie verwenden werden, sind PER (Person), LOC (Ort), CORP (Unternehmen), CW (kreatives Werk), GRP (Gruppe von Personen) und PROD (Produkt). Es kann vorkommen, dass Sie mehrteilige Entitäten finden, daher stellen Sie bitte sicher, dass jedes Wort der Entität mit dem entsprechenden Präfix ('B' für das erste Wort der Entität, 'I' für jedes nicht initiale Wort der Entität) gekennzeichnet wird. Für Wörter, die nicht Teil einer benannten Entität sind, sollten Sie 'O' zurückgeben. Das Ausgabeformat sollte eine Liste von Tupeln sein, wobei jedes Tupel aus einem Wort aus dem Eingabetext und dem entsprechenden benannten Entitätslabel besteht. \\ \hline
    \mtr{6}{Spanish} & Está trabajando como experto en reconocimiento de entidades con nombre y su tarea es etiquetar un texto determinado con etiquetas de entidades con nombre. Su tarea es identificar y etiquetar cualquier entidad nombrada presente en el texto. Las etiquetas de entidad con nombre que utilizará son PER (persona), LOC (ubicación), CORP (corporación), CW (trabajo creativo), GRP (grupo de personas) y PROD (producto). Es posible que encuentre entidades de varias palabras, así que asegúrese de etiquetar cada palabra de la entidad con el prefijo apropiado ('B' para la primera palabra de la entidad, 'I' para cualquier palabra no inicial de la entidad). Para las palabras que no forman parte de ninguna entidad nombrada, debe devolver 'O'. Su formato de salida debe ser una lista de tuplas, donde cada tupla consta de una palabra del texto de entrada y su correspondiente etiqueta de entidad con nombre. \\ \hline
    \mtr{6}{Persian} & \foreignlanguage{farsi}{متخصص شناسایی نامگذاری شده هستید و وظیفه شما برچسب‌گذاری متن داده شده با برچسب‌های نامگذاری شده است. وظیفه شما شناسایی و برچسب‌گذاری هر موجودیت نامگذاری شده در متن است. برچسب‌های موجودیت نامگذاری شده که شما از آن‌ها استفاده خواهید کرد عبارتند از: PER (شخص)، LOC (موقعیت)، CORP (شرکت)، CW (ایجاد کار)، GRP (گروه افراد) و PROD (محصول). ممکن است با موجودیت‌های چند کلمه‌ای مواجه شوید، بنابراین مطمئن شوید که هر کلمه از موجودیت با پیشوند مناسب ('B' برای اولین کلمه موجودیت، 'I' برای هر کلمه غیر اولیه موجودیت) برچسب‌گذاری شود. برای کلماتی که بخشی از هیچ موجودیت نامگذاری شده‌ای نیستند، باید 'O' بازگردانده شود. قالب خروجی شما باید یک لیست از تاپل‌ها باشد، که هر تاپل شامل یک کلمه از متن و برچسب موجودیت نامگذاری شده متناظر با آن است. برای هر کلمه، برچسب موجودیت نامگذاری شده باید با یکی }\\ \hline
    \mtr{6}{Dutch} & U werkt als expert op het gebied van benoemde entiteitsherkenning en het is uw taak om een bepaalde tekst te labelen met benoemde entiteitslabels. Het is jouw taak om benoemde entiteiten in de tekst te identificeren en te labelen. De benoemde entiteitslabels die u gaat gebruiken zijn PER (persoon), LOC (locatie), CORP (bedrijf), CW (creatief werk), GRP (groep mensen) en PROD (product). U kunt entiteiten met meerdere woorden tegenkomen, dus zorg ervoor dat u elk woord van de entiteit labelt met het juiste voorvoegsel ('B' voor het eerste woord van de entiteit, 'I' voor elk niet-initieel woord van de entiteit). Voor woorden die geen deel uitmaken van een benoemde entiteit, moet u 'O' retourneren. Uw uitvoerformaat moet een lijst met tupels zijn, waarbij elke tupel bestaat uit een woord uit de invoertekst en het bijbehorende benoemde entiteitslabel. \\ \hline
    \mtr{6}{Russian} & \foreignlanguage{russian}{Вы работаете экспертом по распознаванию именованных сущностей, и ваша задача состоит в том, чтобы пометить заданный текст метками именованных сущностей. Ваша задача состоит в том, чтобы возникновение и значение обозначить любые именованные объекты, присутствующие в тексте. Вы сможете использовать метки именных объектов: PER (человек), LOC (местоположение), CORP (корпорация), CW (творческая работа), GRP (группа людей) и PROD (продукт). Вы можете столкнуться с объектом, состоящим из нескольких слов, поэтому не преследуется цель пометить каждое слово объекта соответствующим префиксом («B» для первого слова объекта, «I» для любого неначального слова объекта). Для слов, которые не являются частью какого-либо именованного объекта, вы должны вернуть 'O'. Ваш выходной формат должен быть неожиданным для кортежей, где кортеж состоит из слов из входного текста и подозрения на метки именованного объекта.} \\ \hline
    \mtr{6}{Turkish} & Adlandırılmış bir varlık tanıma uzmanı olarak çalışıyorsunuz ve göreviniz, belirli bir metni adlandırılmış varlık etiketleriyle etiketlemek. Göreviniz, metinde bulunan herhangi bir adlandırılmış varlığı tanımlamak ve etiketlemektir. Kullanacağınız adlandırılmış varlık etiketleri şunlardır: PER (kişi), LOC (konum), CORP (şirket), CW (yaratıcı çalışma), GRP (insan grubu) ve PROD (ürün). Çok kelimeli varlıklarla karşılaşabilirsiniz, bu nedenle varlığın her bir kelimesini uygun önekle etiketlediğinizden emin olun (varlığın ilk kelimesi için 'B', varlığın ilk olmayan herhangi bir kelimesi için 'I'). Herhangi bir adlandırılmış varlığın parçası olmayan kelimeler için 'O' döndürmelisiniz. Çıktı biçiminiz, her bir demetin giriş metnindeki bir kelimeden ve buna karşılık gelen adlandırılmış varlık etiketinden oluştuğu bir demetler listesi olmalıdır. \\ \hline
\end{tabular}
}
\caption{Language-specific task descriptions for the MultiCoNER dataset translated from the English version.}
\label{tab:prompt-multiconer}
\end{table}
